# Supplementary material for: Automated event generation for S-wave quarkonium and leptonium production in NRQCD and NRQED
Source: arXiv:2510.26773 ancillary file (2026-03-01)
Supplement: Supplementary file 1 [file benchmarks.pdf]

# Automated event generation for S-wave quarkonium and leptonium production in NRQCD and NRQED

## – Supplementary Material –

This document presents our extensive benchmarks for the *standalone mode*, comprising 42 different processes that have been tested and validated against **HELAC-Onia**. A selection of these results is showcased in table 4 of the main article.

Table 1 reports the validation test described in detail in section 5 of the article. It shows the squared helicity amplitudes averaged (summed) over the colours and helicities of the initial-state (final-state) particles for a randomly generated physical phase-space point. Only the leading-order contributions with the lowest possible power of the electroweak coupling constant  $\alpha$  are included.

In contrast, table 2 is generated with the additional flag **QCD=99 QED=99** (see footnote 13 in the article), which also incorporates subdominant contributions by including all diagrams of  $\mathcal{O}(\alpha_s^i \alpha^j)$  for a fixed value of  $i + j$ .

| process                                                                 | MG5_aMC<br>HELAC-Onia                                                                                        | $\Delta_{\text{rel.}}$ |
|-------------------------------------------------------------------------|--------------------------------------------------------------------------------------------------------------|------------------------|
| $u\bar{u} \rightarrow \eta_c \left[ {}^1S_0^{[1]} \right] + g$          | $2.3281771700153857 \cdot 10^{-8}$<br>$2.3281771700153804 \cdot 10^{-8}$                                     | $2.2 \cdot 10^{-15}$   |
| $gg \rightarrow \eta_c \left[ {}^1S_0^{[1]} \right] + g$                | $2.8407532009628355 \cdot 10^{-6}$<br>$2.8407532009628347 \cdot 10^{-6}$                                     | $2.2 \cdot 10^{-16}$   |
| $gg \rightarrow J/\psi \left[ {}^3S_1^{[8]} \right] + g$                | $4.132917971335 \cdot 10^{-3}$<br>$4.132917971659 \cdot 10^{-3}$                                             | $7.8 \cdot 10^{-11}$   |
| $gg \rightarrow \eta_b \left[ {}^1S_0^{[1]} \right] + g$                | $7.492524400362391 \cdot 10^{-6}$<br>$7.492524400362391 \cdot 10^{-6}$                                       | $2.2 \cdot 10^{-16}$   |
| $gg \rightarrow \eta_b \left[ {}^1S_0^{[8]} \right] + H$                | $1.754689170164379 \cdot 10^{-19}$<br>$1.754688903414785 \cdot 10^{-19}$                                     | $1.5 \cdot 10^{-7}$    |
| $u\bar{u} \rightarrow \eta_c \left[ {}^1S_0^{[1]} \right] + c\bar{c}$   | $1.381481341714290 \cdot 10^{-12} \text{ GeV}^{-2}$<br>$1.381481341714289 \cdot 10^{-12} \text{ GeV}^{-2}$   | $1.3 \cdot 10^{-15}$   |
| $gg \rightarrow \eta_c \left[ {}^1S_0^{[1]} \right] + c\bar{c}$         | $2.256515686235864 \cdot 10^{-11} \text{ GeV}^{-2}$<br>$2.256515686235860 \cdot 10^{-11} \text{ GeV}^{-2}$   | $1.8 \cdot 10^{-15}$   |
| $u\bar{u} \rightarrow J/\psi \left[ {}^3S_1^{[1]} \right] + c\bar{c}$   | $8.549390730540083 \cdot 10^{-12} \text{ GeV}^{-2}$<br>$8.549390730535086 \cdot 10^{-12} \text{ GeV}^{-2}$   | $5.8 \cdot 10^{-13}$   |
| $u\bar{u} \rightarrow J/\psi \left[ {}^3S_1^{[1]} \right] + gg$         | $2.1349035674107908 \cdot 10^{-13} \text{ GeV}^{-2}$<br>$2.1349035674211568 \cdot 10^{-13} \text{ GeV}^{-2}$ | $4.9 \cdot 10^{-12}$   |
| $gg \rightarrow J/\psi \left[ {}^1S_0^{[8]} \right] + \gamma Z$         | $1.419801780011157 \cdot 10^{-16} \text{ GeV}^{-2}$<br>$1.419801072960935 \cdot 10^{-16} \text{ GeV}^{-2}$   | $4.9 \cdot 10^{-7}$    |
| $gg \rightarrow \eta_b \left[ {}^1S_0^{[1]} \right] + u\bar{u}$         | $7.422122222821702 \cdot 10^{-11} \text{ GeV}^{-2}$<br>$7.422122222821713 \cdot 10^{-11} \text{ GeV}^{-2}$   | $1.4 \cdot 10^{-15}$   |
| $gg \rightarrow \eta_b \left[ {}^1S_0^{[1]} \right] + gg$               | $3.945645822682013 \cdot 10^{-9} \text{ GeV}^{-2}$<br>$3.945645822682023 \cdot 10^{-9} \text{ GeV}^{-2}$     | $2.6 \cdot 10^{-15}$   |
| $gg \rightarrow B_c^+ \left[ {}^1S_0^{[1]} \right] + b\bar{c}$          | $3.781983565900759 \cdot 10^{-12} \text{ GeV}^{-2}$<br>$3.781983565900755 \cdot 10^{-12} \text{ GeV}^{-2}$   | $1.1 \cdot 10^{-15}$   |
| $u\bar{u} \rightarrow B_c^+ \left[ {}^3S_1^{[8]} \right] + b\bar{c}$    | $6.87392368906369 \cdot 10^{-14} \text{ GeV}^{-2}$<br>$6.87392368906585 \cdot 10^{-14} \text{ GeV}^{-2}$     | $3.1 \cdot 10^{-13}$   |
| $gg \rightarrow B_c^+ \left[ {}^3S_1^{[8]} \right] + b\bar{c}$          | $2.623514829803796 \cdot 10^{-13} \text{ GeV}^{-2}$<br>$2.623514829804791 \cdot 10^{-13} \text{ GeV}^{-2}$   | $3.8 \cdot 10^{-13}$   |
| $u\bar{u} \rightarrow B_c^{*+} \left[ {}^3S_1^{[1]} \right] + b\bar{c}$ | $1.715497539525171 \cdot 10^{-11} \text{ GeV}^{-2}$<br>$1.715497539525771 \cdot 10^{-11} \text{ GeV}^{-2}$   | $3.5 \cdot 10^{-13}$   |
| $u\bar{u} \rightarrow \eta_c \left[ {}^1S_0^{[1]} \right] + ggg$        | $4.05096985838911 \cdot 10^{-14} \text{ GeV}^{-4}$<br>$4.05096985838916 \cdot 10^{-14} \text{ GeV}^{-4}$     | $1.0 \cdot 10^{-14}$   |

|                                                                                                                                        |                                                                                                              |                      |
|----------------------------------------------------------------------------------------------------------------------------------------|--------------------------------------------------------------------------------------------------------------|----------------------|
| $gg \rightarrow \eta_c \left[ {}^1S_0^{[1]} \right] + ggg$                                                                             | $5.3063891680528514 \cdot 10^{-11} \text{ GeV}^{-4}$<br>$5.3063891680527945 \cdot 10^{-11} \text{ GeV}^{-4}$ | $1.1 \cdot 10^{-14}$ |
| $gg \rightarrow \eta_c \left[ {}^1S_0^{[8]} \right] + ggg$                                                                             | $7.53882646402403 \cdot 10^{-13} \text{ GeV}^{-4}$<br>$7.53882646469246 \cdot 10^{-13} \text{ GeV}^{-4}$     | $8.9 \cdot 10^{-11}$ |
| $u\bar{u} \rightarrow J/\psi \left[ {}^3S_1^{[1]} \right] + ggg$                                                                       | $1.259893829577019 \cdot 10^{-14} \text{ GeV}^{-4}$<br>$1.259893829578596 \cdot 10^{-14} \text{ GeV}^{-4}$   | $1.3 \cdot 10^{-12}$ |
| $gg \rightarrow \eta_c \left[ {}^1S_0^{[1]} \right] + \eta_c \left[ {}^1S_0^{[1]} \right]$                                             | $2.0249798013364516 \cdot 10^{-14}$<br>$2.0249798013364402 \cdot 10^{-14}$                                   | $5.6 \cdot 10^{-15}$ |
| $gg \rightarrow \eta_b \left[ {}^1S_0^{[1]} \right] + \eta_c \left[ {}^1S_0^{[1]} \right]$                                             | $1.482579515408239 \cdot 10^{-13}$<br>$1.482579515408241 \cdot 10^{-13}$                                     | $8.9 \cdot 10^{-16}$ |
| $gg \rightarrow \eta_b \left[ {}^1S_0^{[1]} \right] + \eta_b \left[ {}^1S_0^{[1]} \right]$                                             | $1.407485887176679 \cdot 10^{-13}$<br>$1.407485887176677 \cdot 10^{-13}$                                     | $8.9 \cdot 10^{-16}$ |
| $gg \rightarrow \eta_b \left[ {}^1S_0^{[1]} \right] + \eta_b \left[ {}^1S_0^{[8]} \right]$                                             | $1.9756046682407265 \cdot 10^{-15}$<br>$1.9756046682408094 \cdot 10^{-15}$                                   | $4.2 \cdot 10^{-14}$ |
| $gg \rightarrow J/\psi \left[ {}^3S_1^{[8]} \right] + J/\psi \left[ {}^3S_1^{[8]} \right] + g$                                         | $7.885078771250576 \cdot 10^{-11} \text{ GeV}^{-2}$<br>$7.885078772660938 \cdot 10^{-11} \text{ GeV}^{-2}$   | $1.8 \cdot 10^{-10}$ |
| $gg \rightarrow \eta_b \left[ {}^1S_0^{[1]} \right] + \eta_c \left[ {}^1S_0^{[1]} \right] + H$                                         | $6.165152391422585 \cdot 10^{-25} \text{ GeV}^{-2}$<br>$6.165151454119377 \cdot 10^{-25} \text{ GeV}^{-2}$   | $1.5 \cdot 10^{-7}$  |
| $gg \rightarrow \eta_b \left[ {}^1S_0^{[1]} \right] + \eta_b \left[ {}^1S_0^{[1]} \right] + H$                                         | $5.068831723452297 \cdot 10^{-25} \text{ GeV}^{-2}$<br>$5.068830952821875 \cdot 10^{-25} \text{ GeV}^{-2}$   | $1.5 \cdot 10^{-7}$  |
| $gg \rightarrow \eta_b \left[ {}^1S_0^{[1]} \right] + \eta_b \left[ {}^1S_0^{[8]} \right] + H$                                         | $3.685993076814355 \cdot 10^{-26} \text{ GeV}^{-2}$<br>$3.685992516420316 \cdot 10^{-26} \text{ GeV}^{-2}$   | $1.5 \cdot 10^{-7}$  |
| $gg \rightarrow \eta_b \left[ {}^1S_0^{[1]} \right] + \Upsilon \left[ {}^3S_1^{[1]} \right] + g$                                       | $2.1933776631229393 \cdot 10^{-17} \text{ GeV}^{-2}$<br>$2.1933776631207314 \cdot 10^{-17} \text{ GeV}^{-2}$ | $1.0 \cdot 10^{-12}$ |
| $gg \rightarrow \Upsilon \left[ {}^3S_1^{[1]} \right] + \Upsilon \left[ {}^3S_1^{[8]} \right] + H$                                     | $4.753109487454247 \cdot 10^{-21} \text{ GeV}^{-2}$<br>$4.75310876482473 \cdot 10^{-21} \text{ GeV}^{-2}$    | $1.5 \cdot 10^{-7}$  |
| $gg \rightarrow J/\psi \left[ {}^3S_1^{[1]} \right] + \Upsilon \left[ {}^3S_1^{[1]} \right] + J/\psi \left[ {}^3S_1^{[8]} \right]$     | $2.510898856056359 \cdot 10^{-27} \text{ GeV}^{-2}$<br>$2.510898865795660 \cdot 10^{-27} \text{ GeV}^{-2}$   | $3.9 \cdot 10^{-9}$  |
| $gg \rightarrow \Upsilon \left[ {}^3S_1^{[1]} \right] + \Upsilon \left[ {}^3S_1^{[1]} \right] + \Upsilon \left[ {}^3S_1^{[1]} \right]$ | numerical zero<br>numerical zero                                                                             |                      |
| $e^+e^- \rightarrow J/\psi \left[ {}^3S_1^{[1]} \right] + gg$                                                                          | $1.843805235534046 \cdot 10^{-14} \text{ GeV}^{-2}$<br>$1.843804974567257 \cdot 10^{-14} \text{ GeV}^{-2}$   | $1.4 \cdot 10^{-7}$  |
| $e^+e^- \rightarrow J/\psi \left[ {}^1S_0^{[8]} \right] + c\bar{c}$                                                                    | $1.350294584265 \cdot 10^{-15} \text{ GeV}^{-2}$<br>$1.350294377299 \cdot 10^{-15} \text{ GeV}^{-2}$         | $1.5 \cdot 10^{-7}$  |
| $\gamma g \rightarrow \eta_c \left[ {}^1S_0^{[1]} \right] + gg$                                                                        | $4.928085710474919 \cdot 10^{-13} \text{ GeV}^{-2}$<br>$4.928085710475026 \cdot 10^{-13} \text{ GeV}^{-2}$   | $2.2 \cdot 10^{-14}$ |
| $\gamma g \rightarrow \eta_c \left[ {}^1S_0^{[8]} \right] + gg$                                                                        | $1.0758014357361837 \cdot 10^{-12} \text{ GeV}^{-2}$<br>$1.0758014358315352 \cdot 10^{-12} \text{ GeV}^{-2}$ | $8.9 \cdot 10^{-11}$ |
| $\gamma g \rightarrow \eta_c \left[ {}^1S_0^{[1]} \right] + ggg$                                                                       | $2.168626920441142 \cdot 10^{-14} \text{ GeV}^{-4}$<br>$2.168626920441177 \cdot 10^{-14} \text{ GeV}^{-4}$   | $1.6 \cdot 10^{-14}$ |

Table 1: Benchmark squared amplitudes  $|\mathcal{M}|^2$  (as defined in Eq. 5.1 in the article) in the *standalone mode* for selected partonic processes relevant for various collider types, evaluated at random physical phase-space points. We compare **MG5\_aMC** (top) calculations against **HELAC-Onia** (bottom). The last column of the table shows the relative deviation, as defined in Eq. 5.2.

| process                                                            | MG5_aMC                                             | $\Delta_{\text{rel.}}$ |
|--------------------------------------------------------------------|-----------------------------------------------------|------------------------|
|                                                                    | HELAC-Onia                                          |                        |
| $u\bar{u} \rightarrow B_c^{*+} [^3S_1^{[1]}] + b\bar{c}$           | $1.675806738379 \cdot 10^{-11} \text{ GeV}^{-2}$    | $1.2 \cdot 10^{-7}$    |
|                                                                    | $1.675806931592 \cdot 10^{-11} \text{ GeV}^{-2}$    |                        |
| $gg \rightarrow J/\psi [^3S_1^{[1]}] + \Upsilon [^3S_1^{[1]}] + g$ | $1.156767080922 \cdot 10^{-15} \text{ GeV}^{-2}$    | $2.9 \cdot 10^{-7}$    |
|                                                                    | $1.156766744184 \cdot 10^{-15} \text{ GeV}^{-2}$    |                        |
| $e^+e^- \rightarrow J/\psi [^3S_1^{[1]}] + c\bar{c}$               | $1.69614917552181 \cdot 10^{-10} \text{ GeV}^{-2}$  | $7.7 \cdot 10^{-7}$    |
|                                                                    | $1.69614787531221 \cdot 10^{-10} \text{ GeV}^{-2}$  |                        |
| $e^+e^- \rightarrow J/\psi [^1S_0^{[8]}] + c\bar{c}$               | $1.304158214898 \cdot 10^{-15} \text{ GeV}^{-2}$    | $2.6 \cdot 10^{-7}$    |
|                                                                    | $1.304157872301 \cdot 10^{-15} \text{ GeV}^{-2}$    |                        |
| $e^+e^- \rightarrow \eta_c [^1S_0^{[1]}] + ggg$                    | $2.849455205485939 \cdot 10^{-16} \text{ GeV}^{-4}$ | $3.4 \cdot 10^{-7}$    |
|                                                                    | $2.849454233834478 \cdot 10^{-16} \text{ GeV}^{-4}$ |                        |

Table 2: Benchmark squared amplitudes  $|\mathcal{M}|^2$  (as defined in Eq. 5.1 in the article) including the subdominant LO contributions in the *standalone mode* for selected partonic processes relevant for various collider types, evaluated at random physical phase-space points. We compare MG5\_aMC (top) calculations against HELAC-Onia (bottom). The last column of the table shows the relative deviation, as defined in Eq. 5.2.
